# Supplementary material for: Supporting Cross-language Cross-project Bug Localization Using Pre-trained Language Models
Source: arXiv:2407.02732 source file (2024-07-03)
Supplement: Supplementary file 1 [file appendix.tex]

\appendix
\section{Ranking Algorithm: Fine-tuning}

Algorithm~\ref{alg:file_level_evaluation} shows the steps involved in file-level ranking algorithm used for fine-tuning the pretrained language model. 

\begin{algorithm}[ht]
\DontPrintSemicolon
\SetAlgoVlined

\textbf{Input}: Project source files $\mathcal{F} = \{f_1, f_2, ..., f_m\}$, input reports $\mathcal{I} = \{(r_1, F_1), (r_2, F_2), ..., (r_l, F_l) | F_i \subset \mathcal{F}, i = 1, 2, ..., l \}$, an integer numeric $k$, and model parameters \textbf{$\theta$}.

\textbf{Output}: $accuracy\_at\_k$

$\mathsf{E} \leftarrow \{\}$

\For{$f \in \mathcal{F}$}{

	\textbf{e} $\leftarrow$ get\_embedding($f$, \textbf{$\theta$})
	
	$\mathsf{E} \leftarrow \mathsf{E} \cup \{\textbf{e}\}$
}
$\mathsf{R} \leftarrow \{\}$

\For{$(r, F) \in \mathcal{I}$}{

	\textbf{r} $\leftarrow$ get\_embedding($r$, \textbf{$\theta$})
	
	$\mathsf{R} \leftarrow \mathsf{R} \cup \{(\textbf{r}, F)\}$
}
$A \leftarrow \{\}$

\For{$(\textbf{r}, F) \in \mathsf{R}$}{
	
	\textbf{s} $\leftarrow$ cosine\_similarity(\textbf{r}, $\mathsf{E}$) 
	
	$ranked\_file\_list \leftarrow$ descending\_order(\textbf{s}, $\mathcal{F}$)
	
	$rank \leftarrow 0$
	
	\For{(file, score) $\in$ ranked\_file\_list[:k]}{
		
		$rank \leftarrow rank + 1$ 
		
		\If{$file \in F$} {
		
			\textbf{break}
		}
	}
	\eIf{$rank \leq k$} {
		
		$A \leftarrow A$ $\cup$ $\{1\}$
	}{
		$A \leftarrow A$ $\cup$ $\{0\}$
	}
} 
$accuracy\_at\_k \leftarrow$ mean($A$)

\caption{Ranking algorithm for fine-tuning.}
\label{alg:file_level_evaluation}
\end{algorithm}
